# Supplementary material for: Ambient Adventures: Teaching ChatGPT on Developing Complex Stories
Source: arXiv:2308.01734 source file (2023-08-03)
Supplement: Supplementary file 1 [file appendix.tex]

\section{Game Design}
\label{app:games}

\subsection{TextWorld}
\label{app:textworld}
We designed two games in TextWorld \cite{cote2018textworld} text game engine.

\textbf{Housework} is a game where the goal is to finish all tasks and move to the final spot in the house. 
The player starts in certain room within the house and has the option to move around to other rooms to finish the tasks sequentially. The player is able to determine whether current state of the object is correct. If not, the player will check the states of related objects and change those first. The layout of the game is shown in Fig.1.
The layout of the game is shown in Fig.\ref{fig:house_map}.

The game score is obtained when the player finish the single task or reach the win state.
When the player consumes ``\texttt{bananas}" in kitchen, the game ends with a game score: $5$.

\textit{Exemplar story} for experiments in Section~\ref{sec:textgame} is: ``
To water the plant in patio, I need to fill the kettle in the Kitchen. Once I have filled the kettle, I will water the plant.''

Game scores designed for Section~\ref{sec:textgame} are as follows: 
\begin{itemize}
    \item Score 2: \texttt{kettle} is filled; 
    \item Score 2: \texttt{plant} is irrigated.
\end{itemize}

\begin{figure}[tbh!]
    \centering
\includegraphics[width=\linewidth]{figures/appendix/housework.png}
    \caption{Layout of game ``Housework''.}
    \label{fig:house_map}
\end{figure}

\newpage
\section{ChatGPT}
\subsection{Prompts and Training Samples}
\begin{figure}[h]
    \centering
    \includegraphics[width=8cm]{figures/appendix/prompts.png}
    \caption{Prompts Given to ChatGPT Throughout}
    \label{fig:prompts}
\end{figure}
\begin{figure}[h]
    \centering
    \includegraphics[width=8cm]{figures/appendix/training.png}
    \caption{Example of Training Sample}
    \label{fig:training}
\end{figure}
\subsection{Real World Navigation of ChatGPT Story}
This is the implementation of the ChatGPT story within the text game. To make all actions executable, navigational steps are appended for the robot to maneuver around the text world. Refer to Table 1 and for the original story before navigational steps were added.
\begin{table}[h]
\centering
\footnotesize
\setlength\tabcolsep{0.1pt} %
\begin{tabular}{p{0.99\linewidth}}
\toprule
\textbf{Real-World Translation Example:} 1. Wear clothes 2. Open nightstand 3. Go south 4. Go east 5. Use broom 6. Go west 7. Go north 8. Open dresser 9. Go south 10. Go east. 11. Use broom 12. Go west 13. Go north 14. Open dresser 15. Go south 16. Go east 17. Use broom
\bottomrule
\end{tabular}
\caption{Real-World Translation With Navigation
}
\label{tab:ex_navigation_chatgpt}
\end{table}
